# Supplementary material for: An Early Warning of Emerging Biosecurity Risks in Frontier LLMs
Source: arXiv:2607.18056 source file (2026-08-06)
Supplement: Supplementary file 1 [file appendix.tex]

\appendix
\section{Appendix}

%%%%%%%%%%%%%%%%%%%%%%%%%%%%%%%%%
